# Supplementary material for: Stability and metallization of solid oxygen under high pressure
Source: arXiv:1812.03112 source file (2019-02-18)
Supplement: Supplementary file 1 [file Supplementary_information_to_Stability_and_metallization_of_solid_oxygen_under_high_pressure.._Elatresh_et_al.pdf]

# Supporting Information Appendix
# For
# Stability and metallization of solid oxygen under high pressure

**Sabri F. Elatresh, and Stanimir A. Bonev**

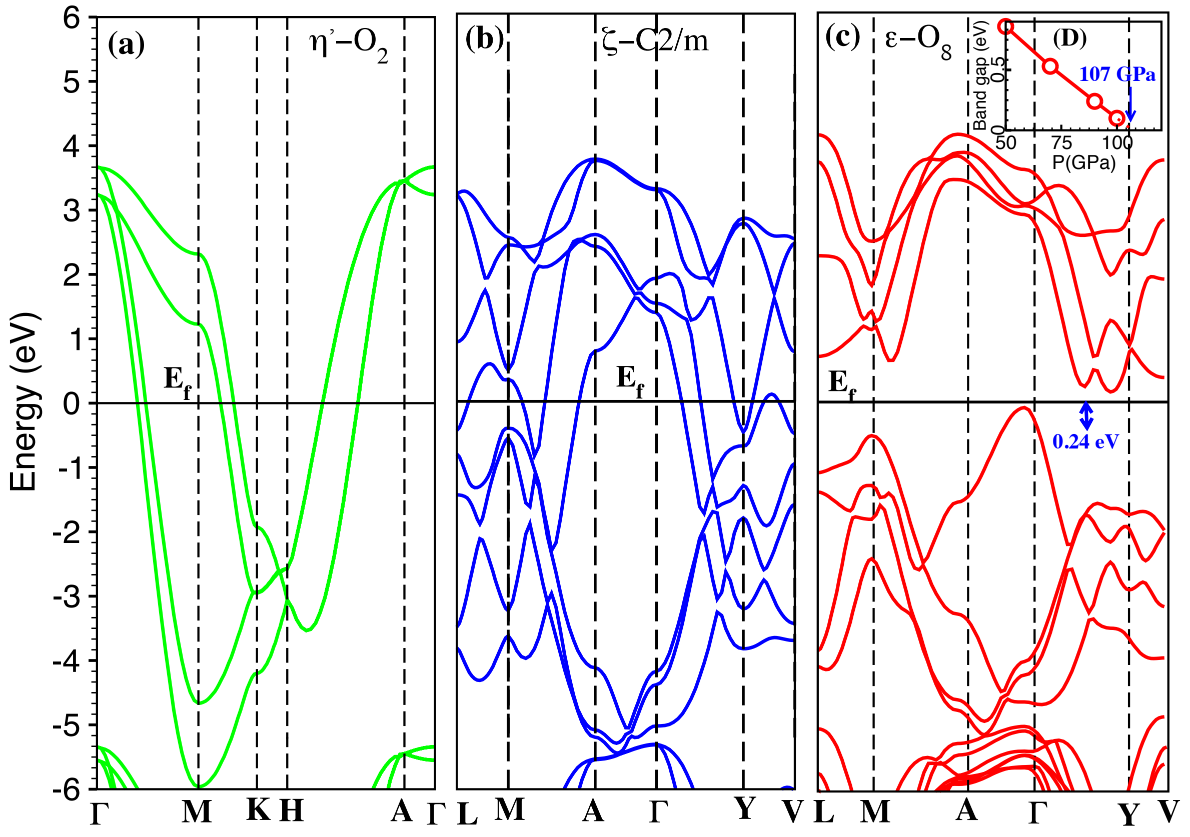


**Fig. S1:** (Color online) HSE06 band structure at 90 GPa for the (a) η′, (b) ζ (C2/m), and (c) $\varepsilon(O_8)$ phases of oxygen. (D) Band gap as a function of pressure.

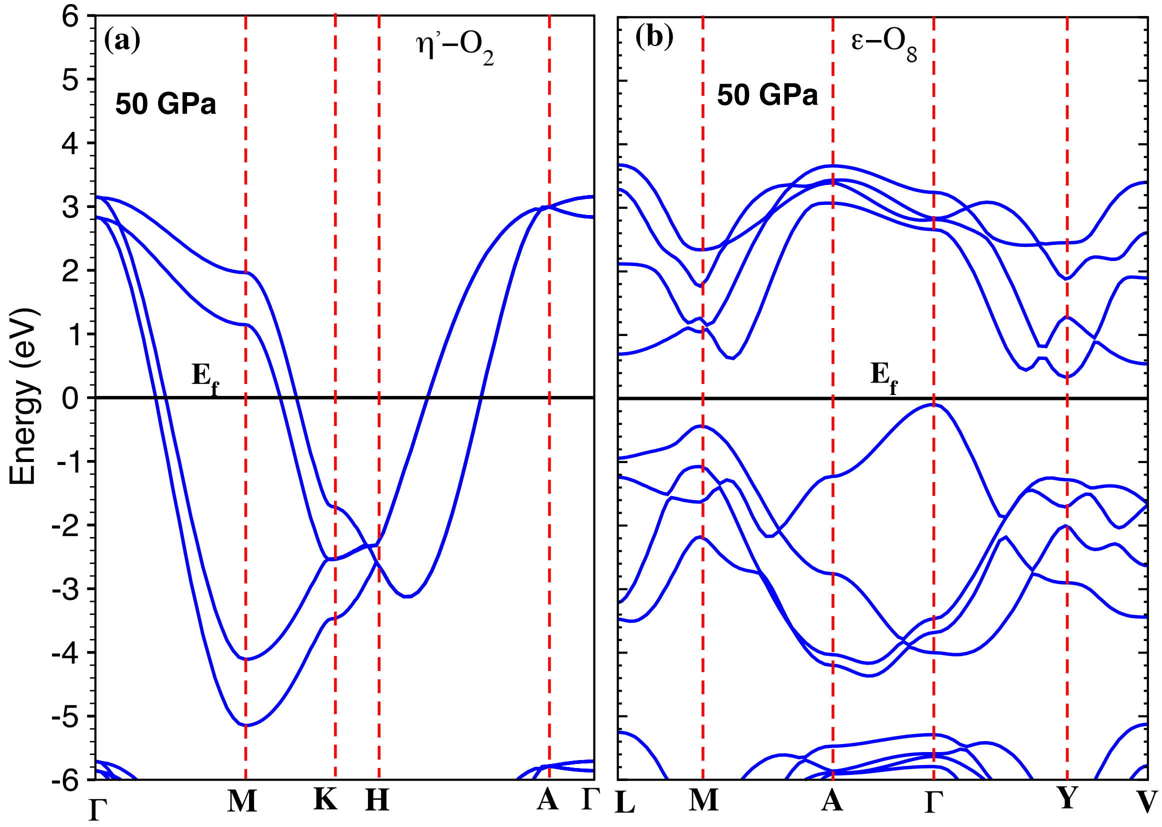


**Fig. S2:** HSE06 band structure at 50 GPa for the (a) η′ and (b) ε($O_8$) phases of oxygen.

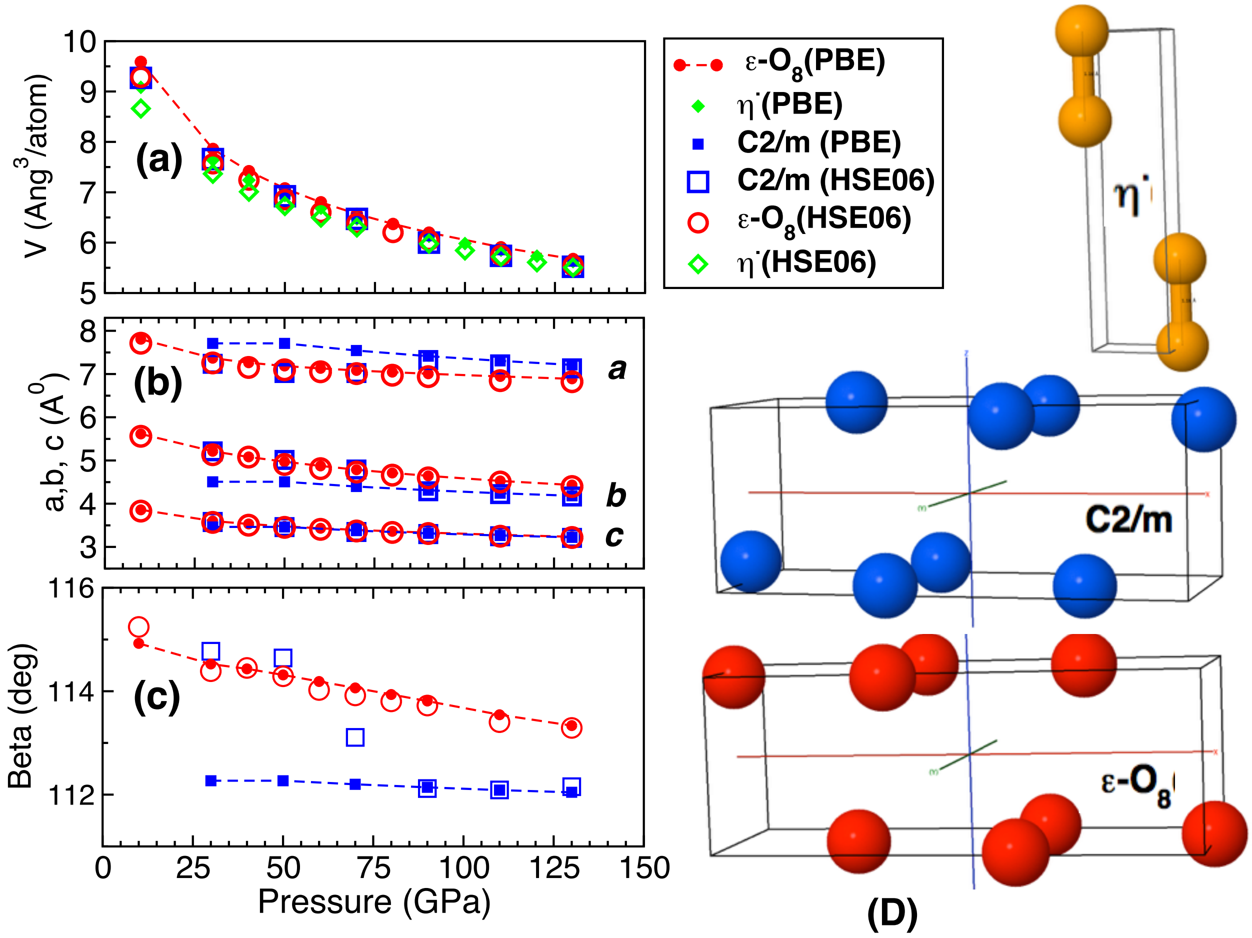


**Fig. S3:** (Color online) Lattice structural parameters from structural optimizations within GGA-PBE and HSE06 as a function of pressure for the $\varepsilon(O_8)$, $\zeta$ (C2/m), and $\eta'$ phases of oxygen. (a) Primitive cells volumes, (b) Primitive cell a, b, and c lattice constants. (c) $\beta$ angle (d) HSE06 relaxed primitive cells at 90 GPa.

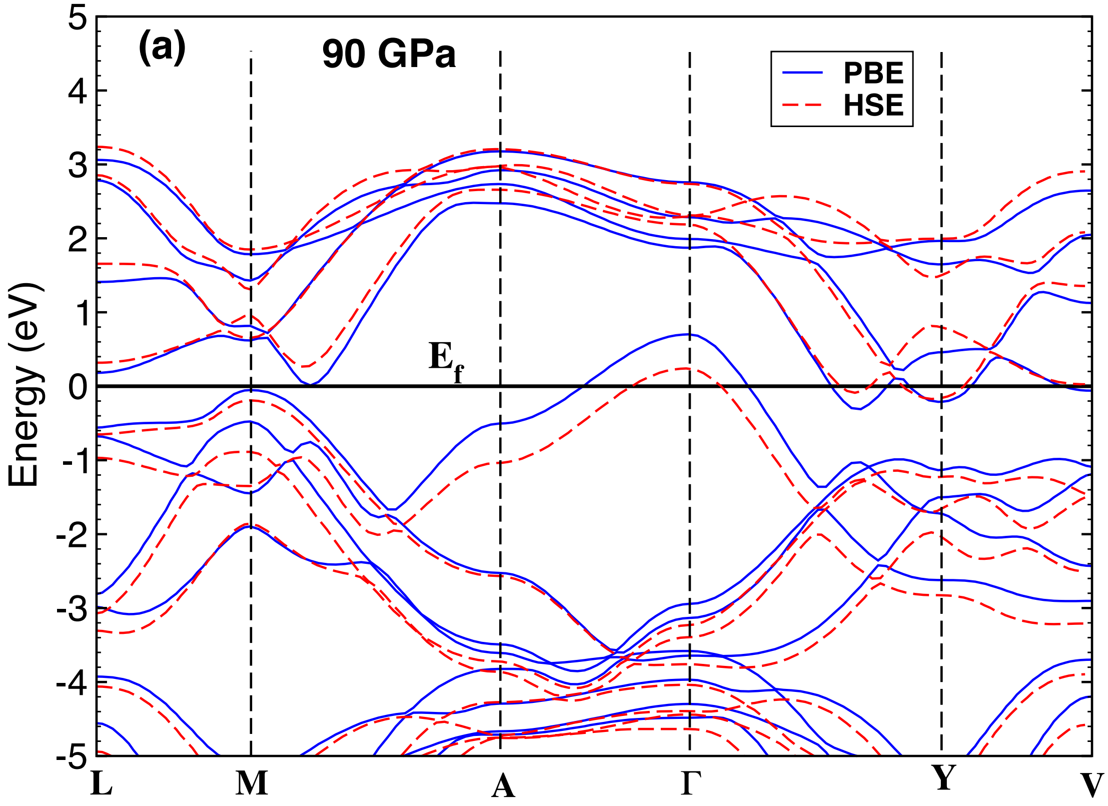


**Fig. S4:** PBE electronic band structure calculations for PBE and HSE optimized ε($O_8$) structure.

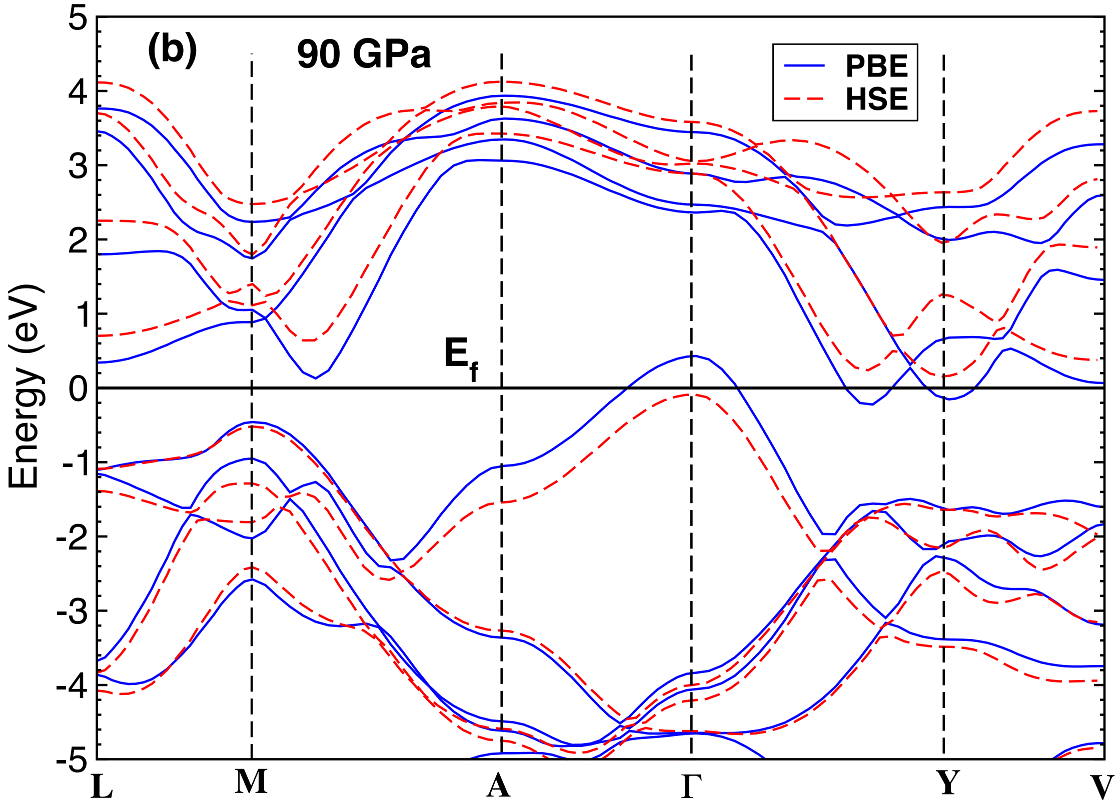


**Fig. S5:** HSE electronic band structure calculations for PBE and HSE optimized ε($O_8$) structure.

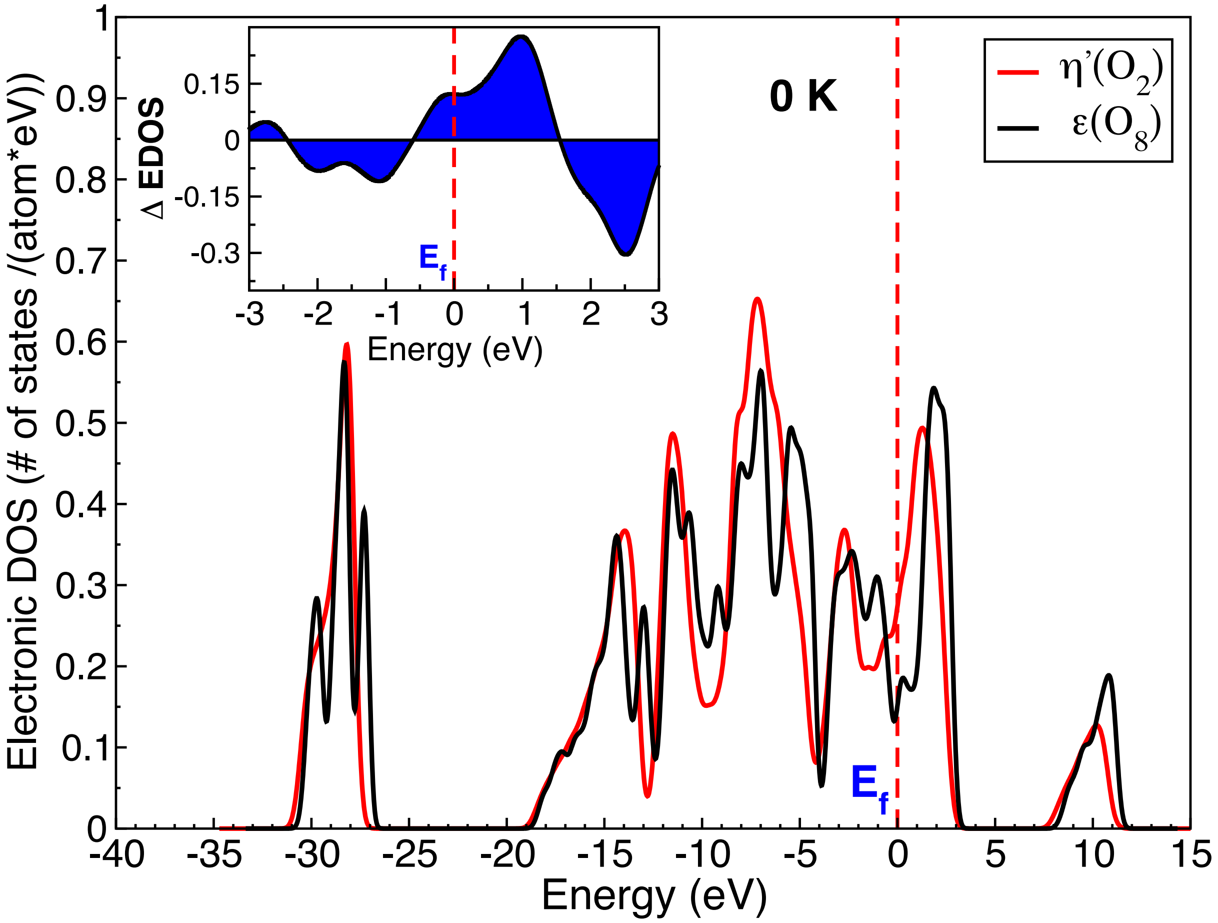


**Fig. S6:** Average electronic density of states (EDOS) of ε($O_8$) and η′ phases at 0~K. The dashed vertical lines represent the location of the Fermi energy. The Inset shows the EDOS difference (Δ EDOS = EDOS (η′)-EDOS (ε($O_8$))).

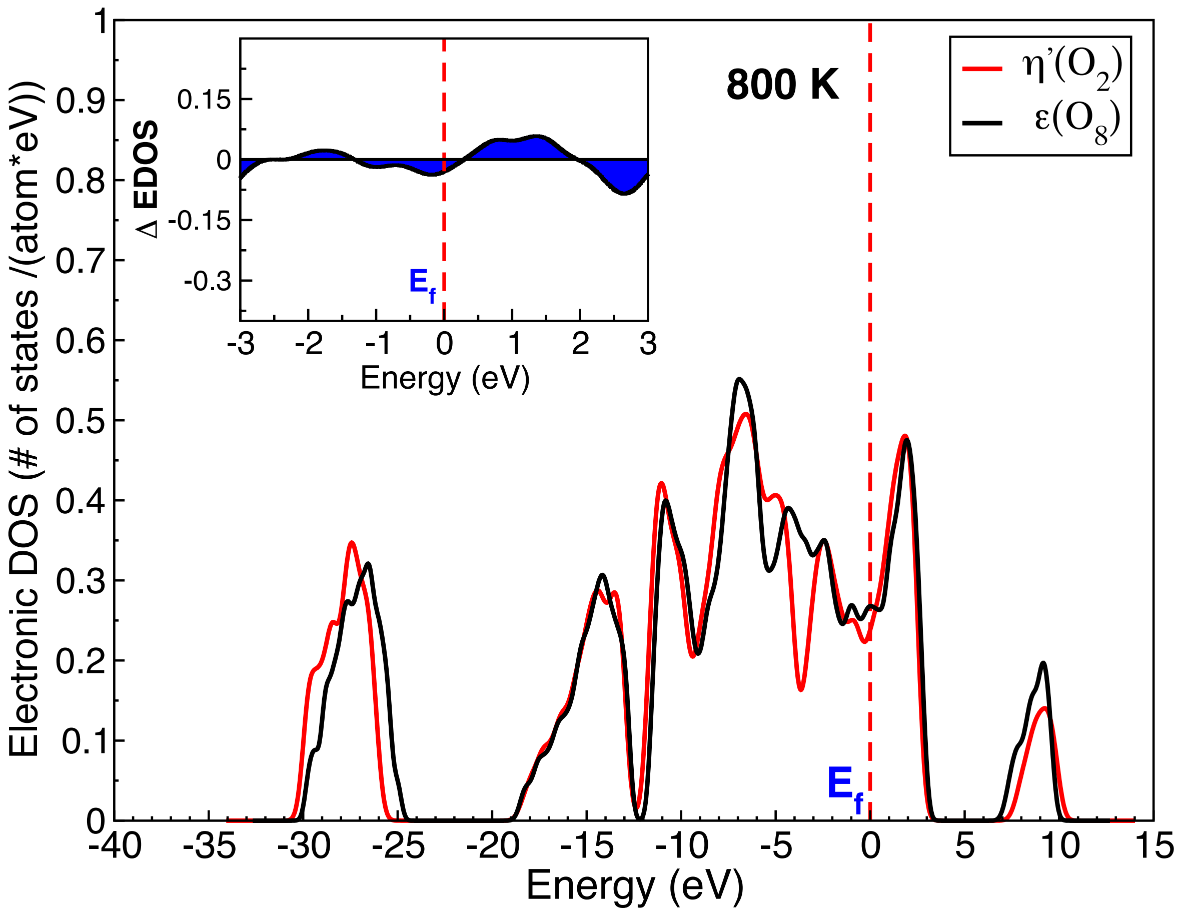


**Fig. S7:** Average electronic density of states of $\varepsilon(O_8)$ and $\eta'$ phases at 800 K. The dashed vertical lines represent location of the Fermi energy. The Inset shows the EDOS difference ($\Delta$ EDOS = EDOS ($\eta'$)-EDOS ($\varepsilon(O_8)$)).
